# Supplementary material for: Explanation-Guided Diagnosis of Machine Learning Evasion Attacks
Source: arXiv:2106.15820 source file (2021-06-30)
Supplement: Supplementary file 1 [file appendix.tex]

\section{Appendix}\label{sec: appendix}

\subsection{Model Architectures and Hyper-Parameters} \label{subsec: a1}
MLP is composed of $5$ hidden layers with the following number of units 32,18,12, 2,1 and a half dropout rate. We use {\em Sigmoid} as an activation function and sparse categorical cross-entropy as loss function. {\em Adam} optimizer is used with $1e-5$ learning rate over $10$ epochs. For LR, we used the default parameters provided by the Scikit-Learn library~\cite{scikit-learn}. RF is used with $random\_state=42$, while all remaining parameters are considered with their default values. For ET, we used $n\_estimators=250$ and $random\_state=0$, with no changes on the other default parameters. DT is used with the default parameters provided in Scikit-Learn. LGBM is provided with EMBER and is pre-trained using 100 trees (31 leaves per tree), resulting in fewer than 10K tunable parameters~\cite{EMBER2018}. Finally, following prior work \cite{DeepMalNet} we train a deep neural network (DNN) over EMBER with $batch\_size = 100$, with 14 dense layers composed of (5608, 5608, 5096, 4608, 4096, 3584, 3072, 2560, 2048, 1536, 1024, 512, 128, 2) units, and a dropout rate of $0.01$ as regularization method. Batch normalization was used in between fully connected layers, to alleviate over-fitting and speed-up DNN model training. {\em Sigmoid} is used as an activation function and binary cross-entropy as loss function. {\em Adam} optimizer is used with $1e-5$ learning rate over $500$ epochs. CNN is composed of 3 convolutional layers with \textit{relu} activation function, one \textit{MaxPooling} layer between the first two convolutional layers and another one after the third convolutional layer. Finally, we add a \textit{Flatten} layer and two final \textit{Dense} layers. We use softmax as the final activation function and SGD optimizer with learning rate $=0.01$ and momentum $=0.9$ over 10 epochs. We adopt the \textit{categorical-crossentropy} as a loss function.
